# Supplementary material for: TeLeS: Temporal Lexeme Similarity Score to Estimate Confidence in End-to-End ASR
Source: arXiv:2401.03251 source file (2024-01-06)
Supplement: Supplementary file 1 [file TASLP_SI_signal_processing.pdf]

**SPECIAL ISSUE**

# **PROPOSAL**

---

## Speech and Language Technologies for Low-resource Languages

**GUEST**

## **EDITORS**

---

### **Dr. Chi Lin**

Senior member of IEEE, ACM, and CCF,  
Associate Professor, Vice Advisor,  
Institute of Intelligent System,  
School of Software,  
Dalian University of Technology,  
Dalian, China.

Email: [clindut@ieee.org](mailto:clindut@ieee.org)

GS: <https://scholar.google.com/citations?user=PVHo2-YAAAAJ>

### **Dr. Chang Wu Yu**

Professor,  
Department of Computer Science and Information Engineering,  
Chung Hua University,  
Hsinchu, Taiwan.

Email: [cwyu@chu.edu.tw](mailto:cwyu@chu.edu.tw)

GS: <https://scholar.google.com/citations?hl=zh-TW&user=M0nQiSwAAAAJ>

### **Dr. Ning Wang**

Assistant Professor,  
Computer Science & Research,  
Rowan University, Glassboro,  
New Jersey, USA.

Email: [wangn@rowan.edu](mailto:wangn@rowan.edu)

GS: <https://scholar.google.com/citations?hl=zh-TW&user=OnrRV0AAAAAJ>

### **Dr. Qiang Lin**

Professor,  
Dalian University of Technology,  
Dalian, China.

Email: [lqchina@dlust.edu.cn](mailto:lqchina@dlust.edu.cn) ; [lqchina@126.com](mailto:lqchina@126.com)

## **SCOPE AND PURPOSE**

---

Speech and language processing is a multi-disciplinary research area that focuses on various aspects of natural language processing and computational linguistics. Speech and language technologies deal with the study of methods and tools to develop innovative paradigms for processing human languages (speech and writing) that can be recognized by machines. Thanks to the incredible advances in machine learning and artificial intelligence techniques that effectively interpret speech and textual sources. In general, speech technologies include a series of artificial intelligence algorithms that enables the computer system to produce, analyze, modify and respond to human speech and texts. It establishes a more natural interaction between the human and the computers and also the translation between all the human languages and effectively analyzes the text and speech. These techniques have significant applications in computational linguistics, natural language processing, computer science, mathematics, speech processing, machine learning, and acoustics. Another important application of this technology is a machine translation of the text and voice.

There exists a huge gap between speech and language processing in low-resource languages as they have lesser computational resources. With the ability to access the vast amount of computational sources from various digital sources, we can resolve numerous language processing problems in real-time with enhanced user experience and productivity measures. Speech and language processing technologies for low-resource languages are still in their infancy. Research in this stream will enhance the likelihood of these languages becoming an active part of our life, as their importance is paramount. Furthermore, the societal shift towards digital media along with spectacular advances in digital media along with processing power, computational storage, and software capabilities with a vision of transferring low-resource computing language resources into efficient computing models.

This special issue aims to explore the language and speech processing technologies to novel computational models for processing speech, text, and language. The novel and innovative solutions focus on content production, knowledge management, and natural communication of the low-resource languages. We welcome researchers and practitioners working in speech and language processing to present their novel and innovative research contributions for this special section.

## **TOPICS INCLUDE,**

## **BUT ARE NOT LIMITED TO:**

---

- Artificial intelligence assisted speech and language technologies for low-resource languages
- Pragmatics for low resource languages
- Emerging trends in knowledge representation for low resource languages
- Machine translation for low resource language processing
- Sentiment and statistical analysis for low resource languages
- Automatic speech recognition and speech technology for low resource languages
- Multimodal analysis for low resource languages
- Information retrieval and extraction of low resource languages
- Augment mining for low resource language processing
- Text summarization and speech synthesis
- Sentence-level semantics for speech recognition

## **TENTATIVE DATES**

---

Submission Deadline:

**30<sup>th</sup> May, 2023**

Authors Notification:

**25<sup>th</sup> July, 2023**

Revised Version Submission:

**29<sup>th</sup> September, 2023**

Final Decision Notification:

**15<sup>th</sup> December, 2023**

## **EXPECTED PAPERS FROM THE, LIST OF COUNTRIES**

---

We are planning to promote the special issue among various research communities across the globe through the mail and other online sources, and we expect submission from the following countries listed below,

|               |                |             |
|---------------|----------------|-------------|
| United States | United Kingdom | Germany     |
| South Korea   | France         | Japan       |
| Egypt         | Taiwan         | China       |
| Jordan        | Italy          | Canada      |
| Australia     | Spain          | Switzerland |
